# Supplementary material for: Pomeranchuk Effect and Tunable Quantum Phase Transitions in 3L-MoTe2/WSe2
Source: arXiv:2203.01010 source file (2022-03-02)
Supplement: Supplementary file 1 [file Supplementary_information.pdf]

# Supplementary Materials for
# "Pomeranchuk Effect and Tunable Quantum Phase Transitions in $3L-MoTe_2/WSe_2$"

Mingjie Zhang[1,2], Xuan Zhao[1,2], Kenji Watanabe[3], Takashi Taniguchi[4], Zheng Zhu[5], Fengcheng Wu[6], Yongqing Li[1,2], Yang Xu[1,*]

[1]Beijing National Laboratory for Condensed Matter Physics, Institute of Physics, Chinese Academy of Sciences, Beijing, China

[2]School of Physical Sciences, University of Chinese Academy of Sciences, Beijing, China

[3]Research Center for Functional Materials, National Institute for Materials Science, Tsukuba, Japan

[4]International Center for Materials Nanoarchitectonics, National Institute for Materials Science, Tsukuba, Japan

[5]Kavli Institute for Theoretical Sciences, University of Chinese Academy of Sciences, Beijing, China

[6]School of Physics and Technology, Wuhan University, Wuhan, China

*Email: yang.xu@iphy.ac.cn

**Sample fabrication and optical measurements**

The $3L-MoTe_2/WSe_2$ device was fabricated using a modified layer-by-layer dry transfer method. All the 2D materials used in the study were mechanically exfoliated from bulk crystals onto silicon substrates with a 300 nm oxide layer. We first picked up a hBN/graphite stack as the bottom gate by a polycarbonate (PC) stamp, and then released the stack onto a silicon substrate. Ti/Pt (1nm/5nm) electrodes were patterned into a quasi-Hall bar geometry on bottom gate dielectric hBN by electron-beam lithography and metallization. The polymer residues on hBN were cleaned using an atomic force microscope (AFM) under the contact mode. The top part of the device was prepared by another PC stamp. A hBN/graphite/hBN/$WSe_2$ stack was first picked up layer by layer in ambient conditions. Then the $MoTe_2$ was exfoliated and transferred in a glovebox with an argon atmosphere to avoid degradation. The oxygen and water levels of the glovebox are both below one part per million (ppm). The size and thickness of top gate graphite,

$WSe_2$ and $MoTe_2$ were carefully selected according to their optical contrast. The monolayer $WSe_2$ and trilayer $MoTe_2$ are angle-aligned utilizing their sharp edges. Finally, the top part of the device was released on the pre-patterned Ti/Pt contacts.

The angle alignment between the trilayer $MoTe_2$ and monolayer $WSe_2$ in the finished device was further verified by angle-resolved optical second-harmonic generation (SHG) measurements. As the odd-layer TMD lacks an inversion center, the second-order optical nonlinearity is allowed. A fiber-based femtosecond laser (central wavelength 780 nm, pulse duration ~100 fs, and repetition rate 100 MHz) was used as the excitation source. The input laser was linearly polarized and a half-wave plate was used to control the relative polarization to the sample orientation. An analyzer was kept at crossed polarization with respect to the excitation light. As shown in Supplementary Figure 7, characteristic sixfold polarization dependences were observed for the two flakes, indicating the same crystal orientation (mismatch less than 1°).

**Transport measurements**

Transport data under in-plane magnetic field and higher temperature (>70 K) were acquired in a He-4 cryostat (base $T$=1.7 K, $B$ up to 9 T). All the other data were acquired in a He-3 cryostat (base $T$=300 mK, $B$ up to 9 T). Measurements were performed using a standard low frequency (9.373Hz) lock-in technique under a small bias voltage (1-2 mV). Voltage drops $V_{xx}$, $V_{xy}$, and source-drain current ($I$) were recorded simultaneously to obtain the corresponding longitudinal and Hall resistances. Both the voltage drops were measured using voltage pre-amplifiers with large input impedance (100 MΩ) to maintain the measurement accuracy. Bottom Pt electrodes (that have large workfunction) and large negative top-gate bias ($V_{tg}$) help to obtain Ohmic hole contacts to the 3L-$MoTe_2$/$WSe_2$.

## Supplementary Figures

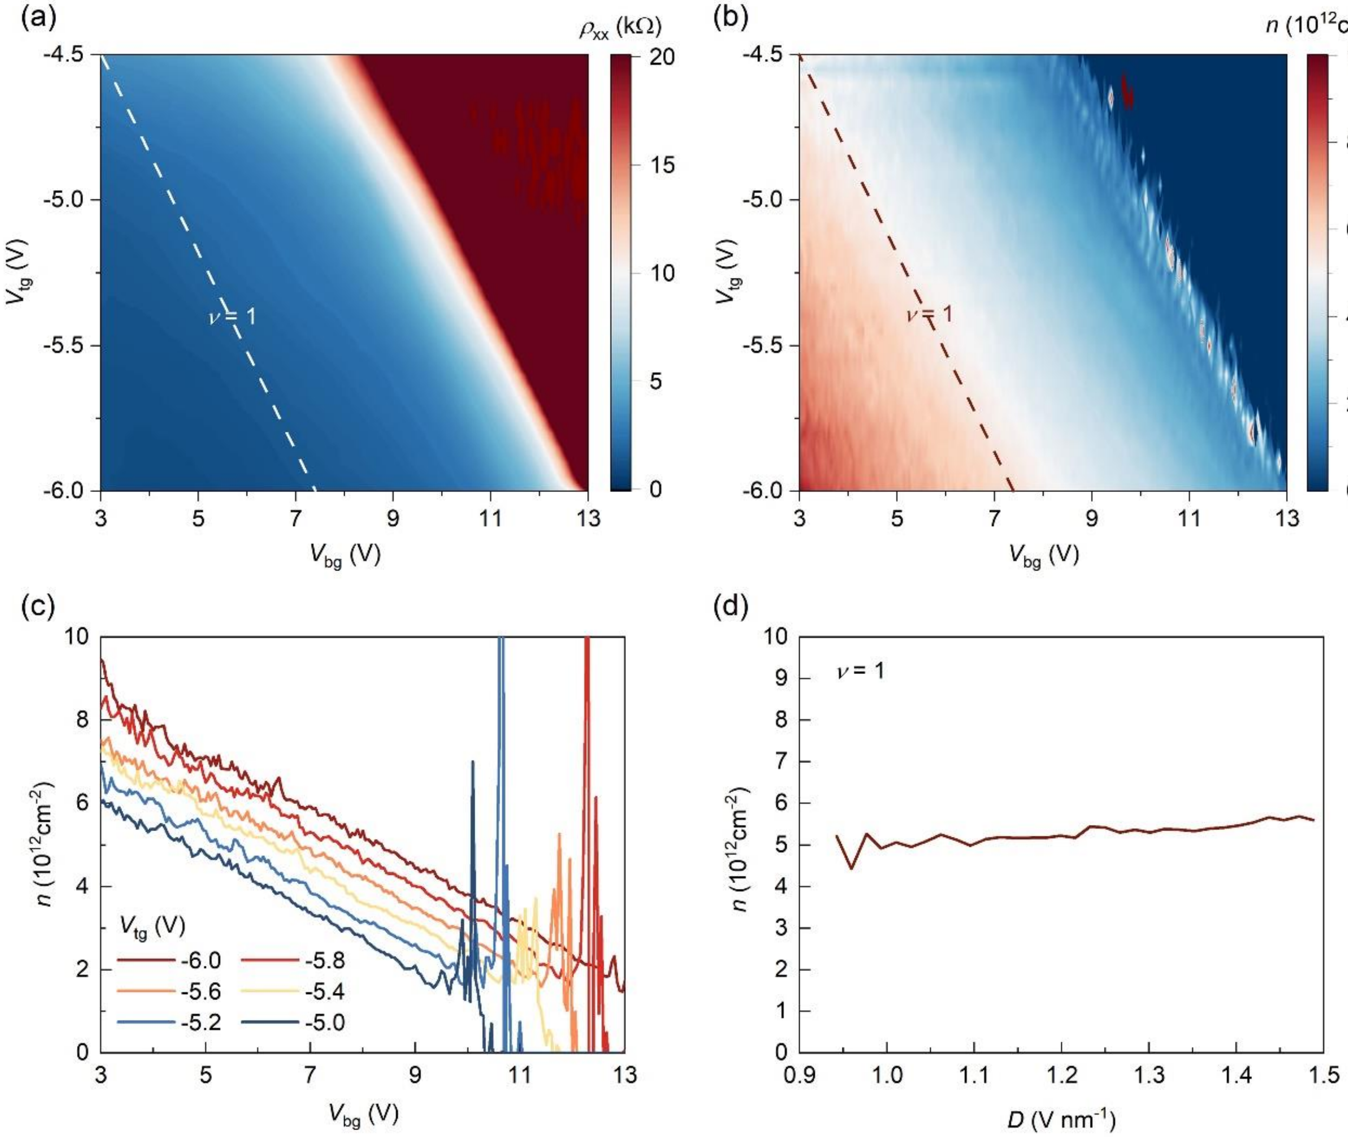


Supplementary Figure 1 | Carrier density measurement at $T$=0.3 K. (a) Longitudinal resistance $\rho_{xx}$ as a function of top and bottom gate voltages ($V_{tg}$ and $V_{bg}$, respectively) at $T$ = 0.3 K and zero magnetic field. Only the $K$ valleys of the topmost $MoTe_2$ layer is populated in this gate-tuned region. The dashed line marks the position of half filling of the first moiré subband ($\nu$=1). No obvious features are observed at $\nu$=1. (b) Gate voltages dependence of carrier density ($n$) at $T$ = 0.3 K. The density is obtained from anti-symmetrized Hall resistance at $B_{\perp} = \pm 1$ T. (c) Linecuts at a few fixed top-gate voltages of **b**. The density $n$ is nearly linearly dependent on both two gates, in good agreement with the expected $n=(C_{tg}V_{tg}+C_{bg}V_{bg})/e$. The $C_{tg}$ and $C_{bg}$ are the geometric capacitances of the top and bottom gates, respectively. The large fluctuation below n<~$2\times10^{12}$ $cm^{-2}$ is due to the large contact resistance near the band edge. (d) The carrier density as a function

of electric displacement field $D$ at $\nu$=1 (along the dashed line in (b)). It is almost independent of the displacement field and equal to the superlattice density. The corresponding Hall mobility is estimated to be ~700 $cm^{-2}$/Vs.

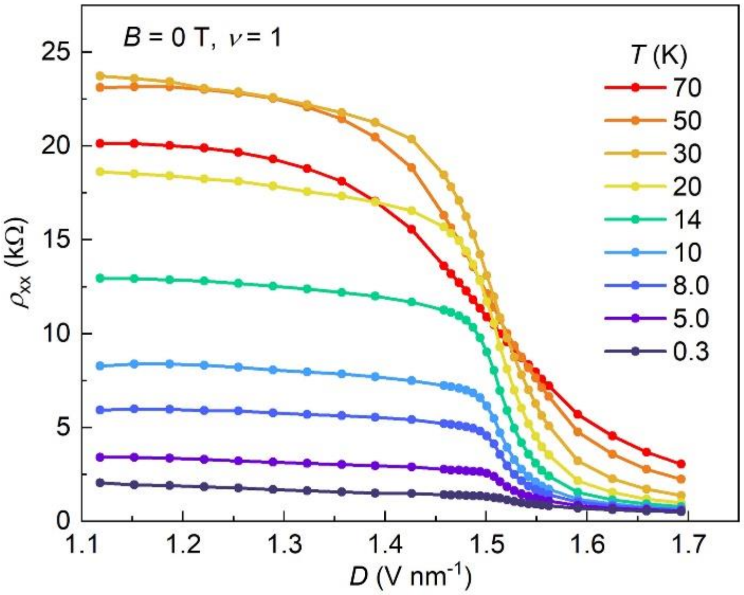


Supplementary Figure 2 | Electric field tuned resistance at $\nu$=1. Electric displacement field $D$ dependence of $\rho_{xx}$ with varying temperature $T$ at $B$ = 0 T and $\nu$ =1. The curves at lower temperatures resemble the $A(D)$ behavior shown in the inset of main-text Fig.2b. Sharp jumps happen near the Lifshitz transition occurring at $D = D_t \approx 1.492\ \mathrm{V\ nm^{-1}}$. The $\rho_{xx}(T)$ changes from a non-monotonic behavior to a monotonic and metallic behavior with a weaker $T$-dependence at larger $D$ fields.

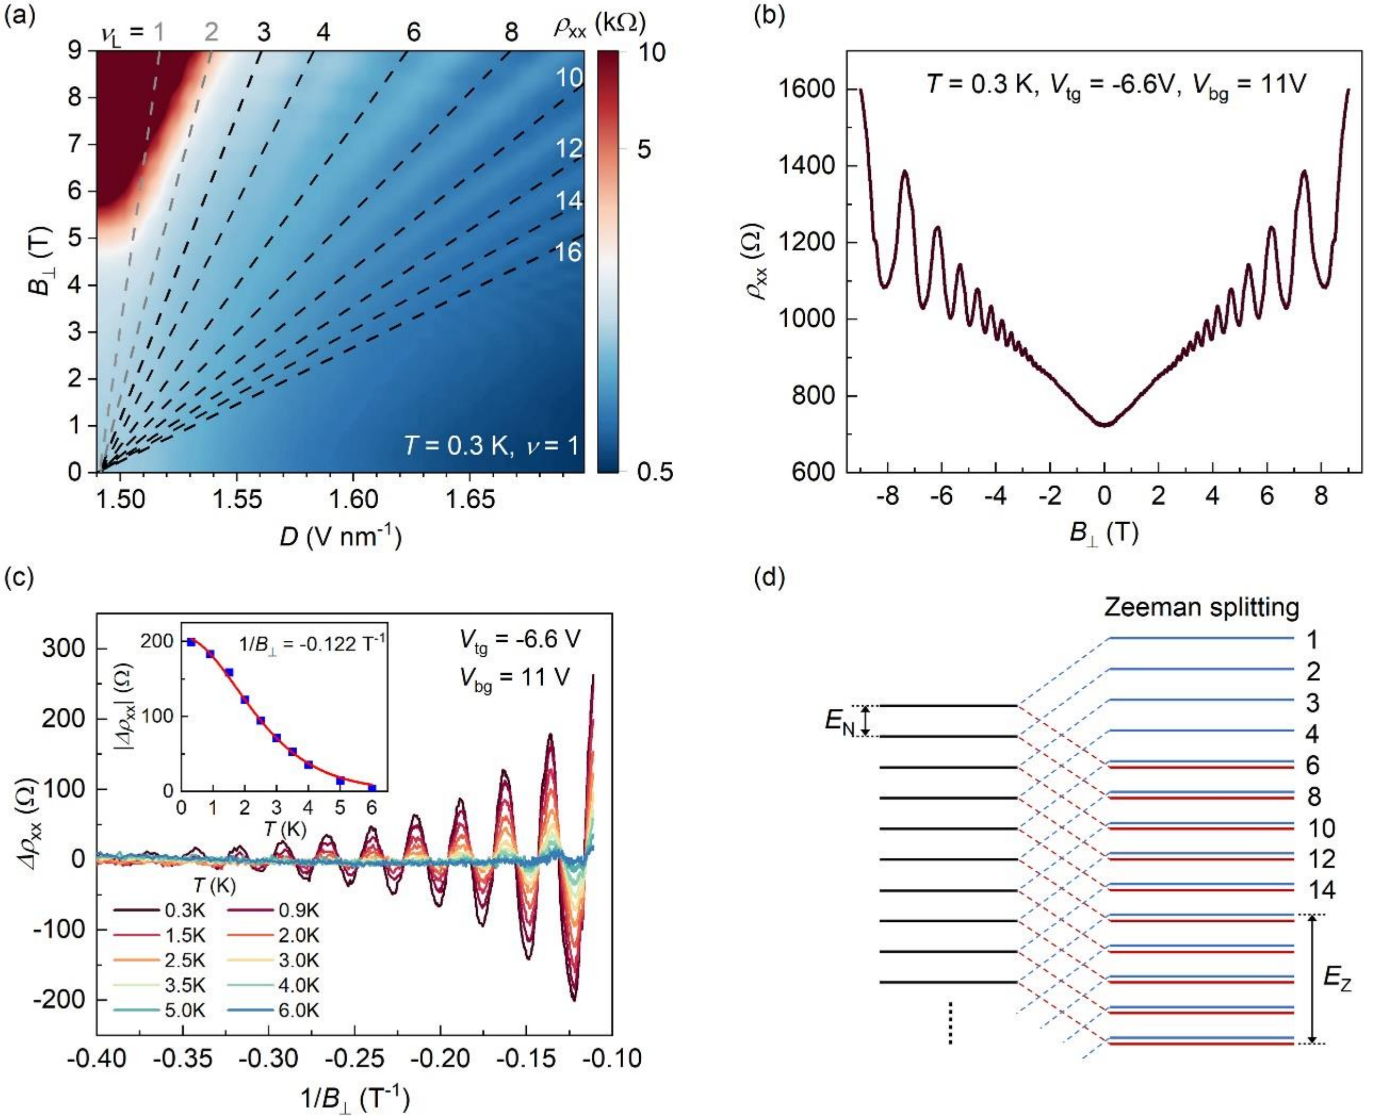


Supplementary Figure 3 | Electric field induced new Fermi surface and quantum oscillations of $WSe_2$. (a) The $\rho_{xx}$ as a function of out-of-plane magnetic field $B_\perp$ and $D$ at $\nu = 1$ and $T = 0.3$ K. The Landau fan is highlighted by the linear dashed lines that diverge from $D_t \approx 1.492$ V nm$^{-1}$, with Landau level filling factors $\nu_L$ labelled accordingly. The Laudau levels are singly degenerate for $\nu_L$=1, 2, 3, 4 and becomes double degenerate for higher ones. The lowest two Landau levels (marked by grey dashed lines) are overwhelmed by the magnetic field induced insulating state at lower $D$ fields. (b) Out-of-plane magnetic field dependence of symmetrized $\rho_{xx}$ at $V_{tg}$ = -6.6 V, $V_{bg}$ = 11 V, and $T$ = 0.3 K. (c) The $\Delta\rho_{xx}$ as a function of $1/B$ at different temperatures, where $\Delta\rho_{xx}$ equals to $\rho_{xx}$ minus a smooth linear baseline. Quantum oscillations disappear near $T$ = 6 K. Inset: temperature dependence of $|\Delta\rho_{xx}|$ at $1/B_\perp$= -0.122 T$^{-1}$. An effective mass $m^* \approx 0.5 m_e$ is extracted by fitting with the standard Lifshitz–Kosevich (LK) theory ($\Delta\rho_{xx} \propto \xi / sinh\, \xi$, where

$\xi = 2\pi^2 k_B T/\hbar\omega_c$ and $\omega_c = eB/m^*$), as shown by the red curve. (d) Schematics showing the Zeeman splitting of the Landau levels, concluded from the experimentally observed Landau level sequences in (a) The $E_N$ and $E_Z$ denote the cyclotron energy and Zeeman energy, respectively, where $E_N = e\hbar B/m^*$ and $E_Z = 2g^*\mu_B B$. From $E_Z \approx 4E_N$, we can estimate the effective Landé $g$-factor $g^* \approx 8$. It is close to the effective mass and $g$-factor found in monolayer $WSe_2$ $K$ valleys [38, 39].

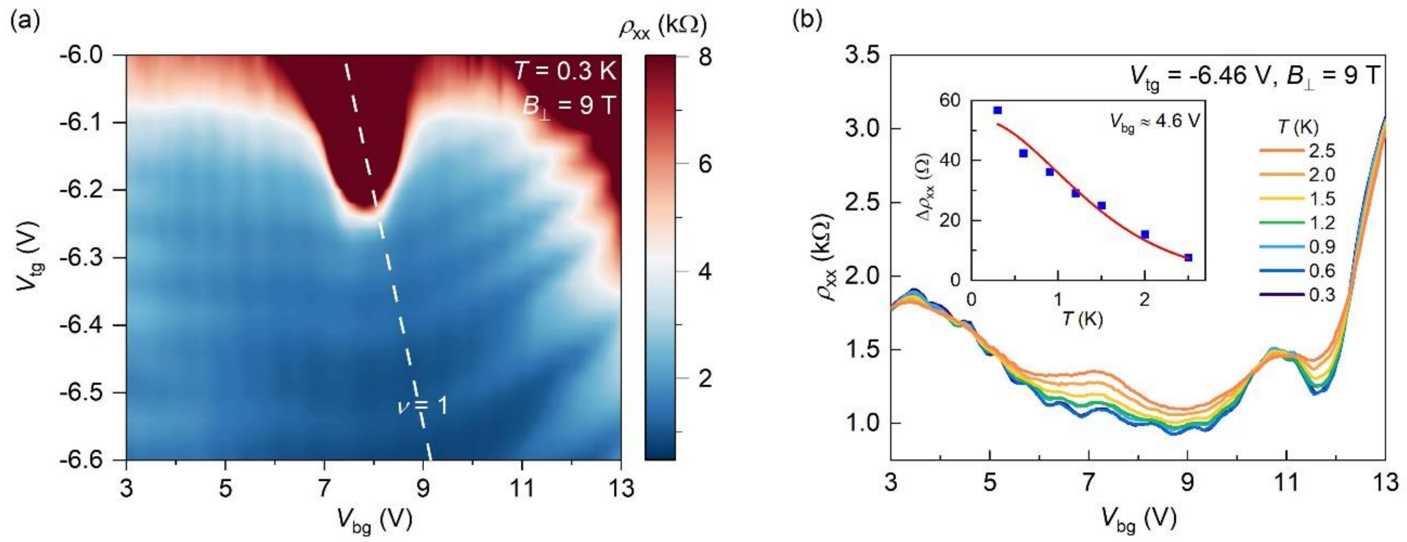


Supplementary Figure 4 | Quantum oscillations from the topmost layer of $MoTe_2$. (a) $\rho_{xx}$ as a function of $V_{tg}$ and $V_{bg}$ at $T$ = 0.3 K and $B_\perp$ = 9 T. The dashed line marks the position of expected half filling $\nu$=1. Landau levels crossings from two sets of quantum oscillations can be observed. The one mainly tuned by $V_{tg}$ holds larger amplitude and comes from the $WSe_2$ monolayer as analysis in the above Fig.3. The other set is mainly tuned by $V_{bg}$, and can be understood to come from the $K$ valleys of the $MoTe_2$, with wavefunctions localized on the topmost layer. (b) The $\rho_{xx}$ as a function of $V_{bg}$ at $V_{tg}$ = -6.46 V and $B_\perp$ = 9 T at different temperatures. The small periodic oscillations almost disappear at $T$ = 2.5 K. Inset: temperature dependence of $\Delta\rho_{xx}$ at $B_\perp$ = 9 T and $V_{bg} \approx$ 4.6 V. $\Delta\rho_{xx}$ is obtained by subtracting a smooth background from $\rho_{xx}$ between $V_{bg}$ = 4.25 V and $V_{bg}$ = 5.75 V. The effective mass extracted from the LK fit (red line) is $m^* \approx 1.0m_e$.

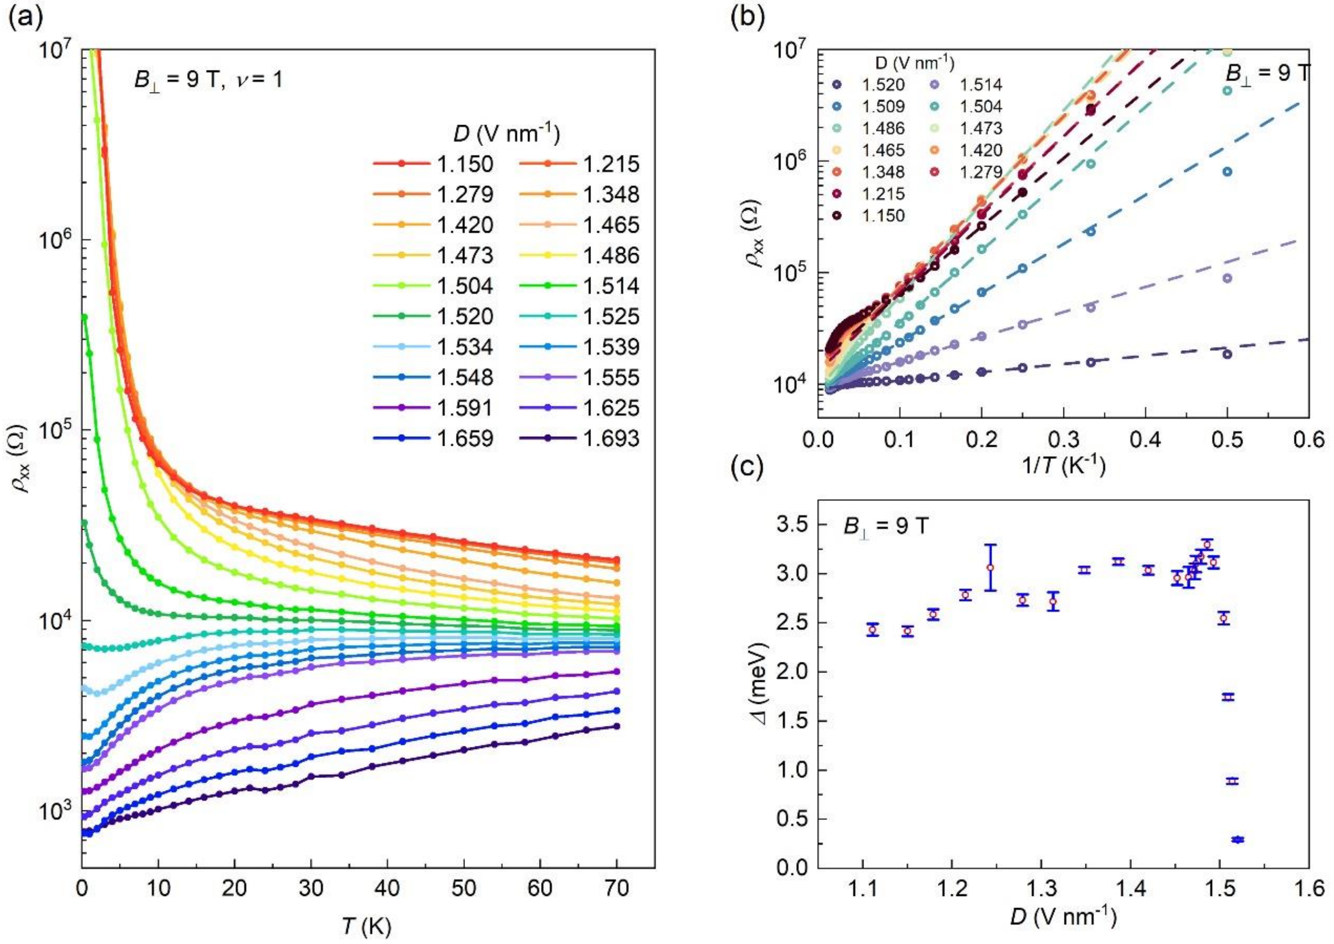


Supplementary Figure 5 | Electric field driven metal-insulator transition at $B_\perp$ = 9 T and $\nu$=1. (a) Temperature dependence of $\rho_{xx}$ at $B_\perp$ = 9 T and $\nu$=1 under varying electric displacement field. As can be seen, the higher temperature (T>10 K) non-monotonic behavior observed at $B_\perp$ = 0 T is absent here. (b) Temperature dependence of $\rho_{xx}$ in an Arrhenius plot. Dashed lines represent Arrhenius fits, which are used to extract activation gap magnitudes Δ for $D$ < 1.52 V nm$^{-1}$. (c) The extracted gap size as a function of displacement field. The gap sharply vanishes near $D$=1.52 V nm$^{-1}$, which is above the Lifshitz transition field $D_t \approx 1.492$ V nm$^{-1}$. As both the $K$ valleys of $MoTe_2$ and $WSe_2$ are populated at $D$>$D_t$, the results potentially indicate an interlayer excitonic insulating state under large magnetic field for $D$ slightly larger than $D_t$. This can also be seen through the intruded insulating region towards the Landau level crossing region in the above Fig. 4a. The observations contrast the $B_\perp$-field tuned MIT shown in Fig.3 or the electric field tuned MIT at zero magnetic field reported for $MoTe_2$/$WSe_2$ homobilayer [28]. Further studies are needed to better understand the electric field driven MIT under external magnetic fields and clarify the correlation between critical electric and magnetic fields.

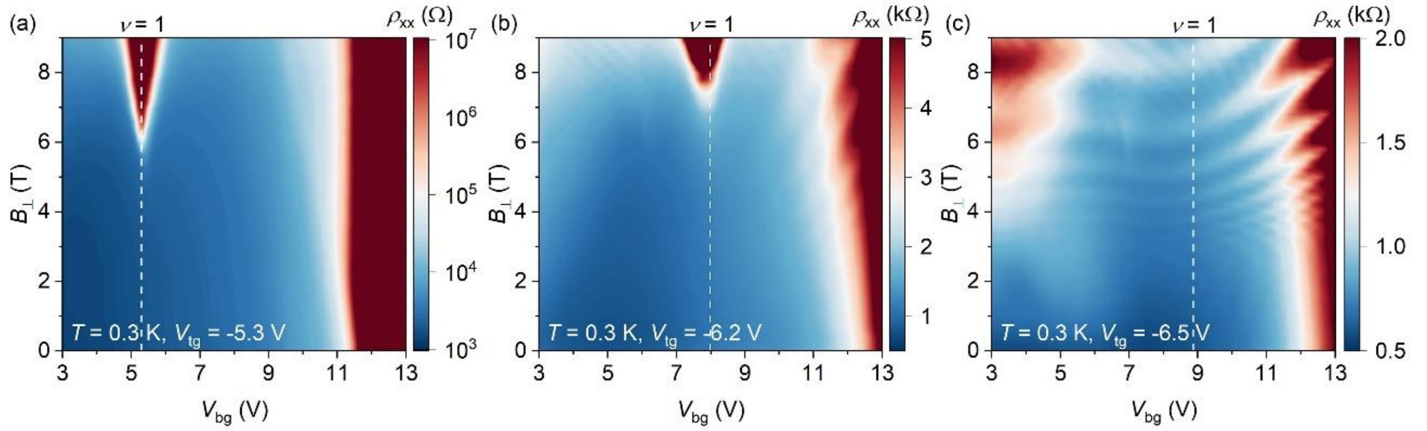


Supplementary Figure 6 | The $\rho_{xx}$ as a function of out-of-plane magnetic field $B_\perp$ and $V_{bg}$ at different $V_{tg}$. (a) At $V_{tg}$ = -5.3 V, corresponding to low displacement field, the magnetic-field-induced metal-insulator transition can be observed at half filling $\nu$=1. (b) At $V_{tg}$ = -6.2 V, near the inflection point of Lifshitz transition, the MIT happens at slightly larger magnetic fields and some quantum oscillation features can be observed. (c) At $V_{tg}$ = -6.5 V, corresponding to high displacement field, Landau levels are clearly resolved, while no magnetic field induced MIT can be observed.

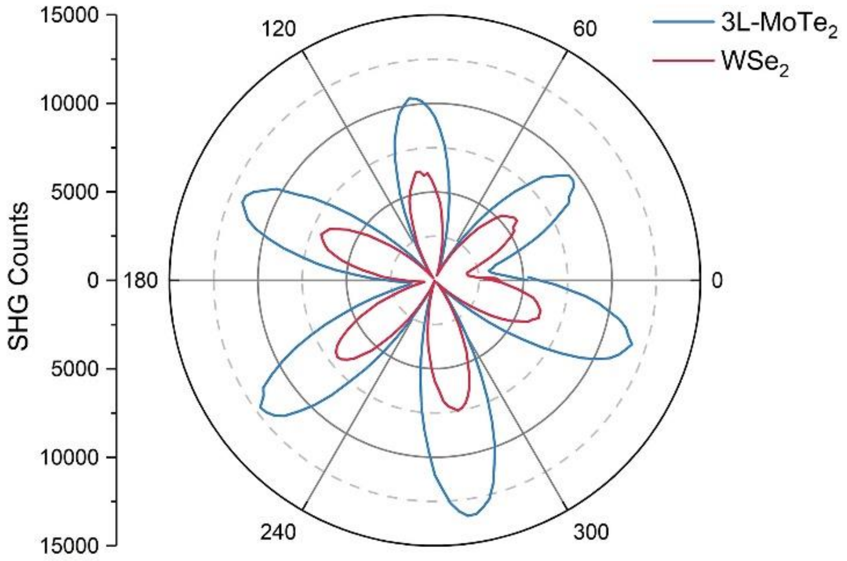


Supplementary Figure 7 | Polarization-dependent SHG measurements. The SHG signals are measured on isolated trilayer $MoTe_2$ and monolayer $WSe_2$, respectively, confirming the crystal alignment (within 1° error) between the two materials.
